# Supplementary material for: DIAMOND: Taming Sample and Communication Complexities in Decentralized Bilevel Optimization
Source: arXiv:2212.02376 source file (2023-01-19)
Supplement: Supplementary file 1 [file Appendix_Proof.tex]

% !TEX root = main.tex

% ----------------------- %
% Have not corrected %
% ----------------------- %

\section{Proof of Theorem~\ref{thm1}} \label{sec: Proof}
\subsection{Step 1: Descent in the iterates of the upper-level function}

\begin{lemma}
    Under Assumptions~\ref{asmp_up} and \ref{asmp_lo}, with $e_{i, t}^{f}$ defined as $e_{i, t}^{f}:=p_{i}\left( x_{i,t},y_{i,t} \right)-\bar{\nabla} f_{i}\left( x_{i,t},y_{i,t} \right)-B_{i}\left( x_{i,t},y_{i,t} \right)$, where $B_{i}\left( x_{i,t},y_{i,t} \right):=\mathbb{E}_{\bar{\xi}_{i}}\left[ \hat{\nabla} f_{i}\left( x_{i,t},y_{i,t};\bar{\xi}_{i} \right) \right]-\bar{\nabla} f_{i}\left( x_{i,t},y_{i,t} \right)$ is the bias in estimating $\bar{\nabla} f_{i}\left( x_{i,t},y_{i,t} \right)$, the following inequality holds for the consecutive iterates of Algorithm~\ref{alg}:
    \begin{equation*}
        \begin{aligned}
            \mathbb{E}\left[ l\left( \bar{x}_{t+1} \right)-l\left( \bar{x}_{t} \right) \right]\le
            & \mathbb{E}\left[ -\frac{\alpha_{t}}{2}\left\|\nabla l\left(\bar{x}_{t}\right)\right\|^{2}-\left(\frac{\alpha_{t}}{2}-\frac{L_{l} \alpha_{t}^{2}}{2}\right)\left\|\bar{u}_{t}\right\|^{2}+\frac{2\alpha_{t}}{m} \sum_{i=1}^{m} L_{l}^{2}\left\|\bar{x}_{t}-x_{i, t}\right\|^{2}\right. \\
            &\left. +\frac{2 \alpha_{t}}{m} \sum_{i=1}^{m}\left\|B_{i, t}\right\|^{2}+\frac{2 \alpha_{t}}{m} \sum_{i=1}^{m} L_{f}^{2}\left\|y_{i, t}^{*}-y_{i, t}\right\|^{2}+\frac{2 \alpha_{t}}{m} \sum_{i=1}^{m}\left\|e_{i, t}^{f}\right\|^{2} \right]
        \end{aligned}
    \end{equation*}
    for all $t\in \left\{ 0,1,\ldots,T-1  \right\}$, where the expectation is w.r.t. the stochasticity of the algorithm.
\end{lemma}

\begin{proof}
\begin{align*}
    \mathbb{E}\left[ l\left(\bar{x}_{t+1}\right)-l\left(\bar{x}_{t}\right) \right]& \stackrel{(a)}{\leq}\mathbb{E}\left[ \left\langle \nabla l\left(\bar{x}_{t}\right), \bar{x}_{t+1}-\bar{x}_{t} \right\rangle+\frac{L_{l}}{2}\left\|\bar{x}_{t+1}-\bar{x}_{t}\right\|^{2} \right]\\
    &\stackrel{(b)}{=}\mathbb{E}\left[ -\alpha_{t}\left\langle \nabla l\left(\bar{x}_{t}\right), \bar{u}_{t} \right\rangle+\frac{L_{l} \alpha_{t}^{2}}{2}\left\| \bar{u}_{t} \right\|^{2} \right] \\
    &=\mathbb{E}\left[ -\frac{\alpha_{t}}{2}\left\|\nabla l\left(\bar{x}_{t}\right)\right\|^{2}-\left(\frac{\alpha_{t}}{2}-\frac{L_{l} \alpha_{t}^{2}}{2}\right)\left\|\bar{u}_{t}\right\|^{2}\right.\\
    &\left.+\frac{\alpha_{t}}{2} \| \nabla l\left(\bar{x}_{t}\right)-\frac{1}{m} \sum_{i=1}^{m} \nabla l_{i}\left(x_{i, t}\right)-\frac{1}{m} \sum_{i=1}^{m} B_{i, t}+\frac{1}{m} \sum_{i=1}^{m} B_{i, t}+\frac{1}{m} \sum_{i=1}^{m} \nabla l_{i}\left(x_{i, t}\right)-\bar{u}_{t} \|^{2} \right]\\
    &\stackrel{(c)}{\leq}\mathbb{E}\left[ -\frac{\alpha_{t}}{2}\left\|\nabla l\left(\bar{x}_{t}\right)\right\|^{2}-\left(\frac{\alpha_{t}}{2}-\frac{L_{l} \alpha_{t}^{2}}{2}\right)\left\|\bar{u}_{t}\right\|^{2}+ \frac{\alpha_{t}}{m} \sum_{i=1}^{m}\left\|\nabla l_{i}\left(\bar{x}_{t}\right)-\nabla l_{i}\left(x_{i, t}\right)-B_{i, t}\right\|^{2}\right.\\
    &\left.+\alpha_{t}\left\|\frac{1}{m} \sum_{i=1}^{m} \nabla l_{i}\left(x_{i, t}\right)+\frac{1}{m} \sum_{i=1}^{m} B_{i, t}-\bar{u}_{t}\right\|^{2} \right]\\
    &\stackrel{(d)}{\leq}\mathbb{E}\left[ -\frac{\alpha_{t}}{2}\left\|\nabla l\left(\bar{x}_{t}\right)\right\|^{2}-\left(\frac{\alpha_{t}}{2}-\frac{L_{l} \alpha_{t}^{2}}{2}\right)\left\|\bar{u}_{t}\right\|^{2}+ \frac{2\alpha_{t}}{m} \sum_{i=1}^{m}\left\|\nabla l_{i}\left(\bar{x}_{t}\right)-\nabla l_{i}\left(x_{i, t}\right)\right\|^{2}\right.\\
    &\left.+\frac{2\alpha_{t}}{m} \sum_{i=1}^{m}\left\|B_{i, t}\right\|^{2}+\alpha_{t}\left\|\frac{1}{m} \sum_{i=1}^{m} \nabla l_{i}\left(x_{i, t}\right)+\frac{1}{m} \sum_{i=1}^{m} B_{i, t}-\bar{u}_{t}\right\|^{2} \right]\\
    &\stackrel{(e)}{\leq}\mathbb{E}\left[ -\frac{\alpha_{t}}{2}\left\|\nabla l\left(\bar{x}_{t}\right)\right\|^{2}-\left(\frac{\alpha_{t}}{2}-\frac{L_{l} \alpha_{t}^{2}}{2}\right)\left\|\bar{u}_{t}\right\|^{2}+ \frac{2\alpha_{t}}{m} \sum_{i=1}^{m}L_{l}^{2}\left\|\bar{x}_{t}-x_{i, t}\right\|^{2}\right.\\
    &\left.+\frac{2\alpha_{t}}{m} \sum_{i=1}^{m}\left\|B_{i, t}\right\|^{2}+\alpha_{t}\left\|\frac{1}{m} \sum_{i=1}^{m} \nabla l_{i}\left(x_{i, t}\right)+\frac{1}{m} \sum_{i=1}^{m} B_{i, t}-\bar{u}_{t}\right\|^{2} \right]\\
    &\stackrel{(f)}{\leq}\mathbb{E}\left[ -\frac{\alpha_{t}}{2}\left\|\nabla l\left(\bar{x}_{t}\right)\right\|^{2}-\left(\frac{\alpha_{t}}{2}-\frac{L_{l} \alpha_{t}^{2}}{2}\right)\left\|\bar{u}_{t}\right\|^{2}+ \frac{2\alpha_{t}}{m} \sum_{i=1}^{m}L_{l}^{2}\left\|\bar{x}_{t}-x_{i, t}\right\|^{2}\right.\\
    &\left.+\frac{2\alpha_{t}}{m} \sum_{i=1}^{m}\left\|B_{i, t}\right\|^{2}+\frac{2 \alpha_{t}}{m} \sum_{i=1}^{m}\left\|\bar{\nabla} f_{i}\left(x_{i,t}, y_{i, t}^{*}\right)-\bar{\nabla} f_{i}\left(x_{i,t}, y_{i, t}\right)\right\|^{2}\right.\\
    &\left.+2 \alpha_{t}\left\|\frac{1}{m} \sum_{i=1}^{m} \bar{\nabla} f_{i}\left(x_{i, t}, y_{i, t}\right)+\frac{1}{m} \sum_{i=1}^{m} B_{i, t}-\bar{u}_{t}\right\|^{2} \right]\\
    &\stackrel{(g)}{\leq}\mathbb{E}\left[ -\frac{\alpha_{t}}{2}\left\|\nabla l\left(\bar{x}_{t}\right)\right\|^{2}-\left(\frac{\alpha_{t}}{2}-\frac{L_{l} \alpha_{t}^{2}}{2}\right)\left\|\bar{u}_{t}\right\|^{2}+ \frac{2\alpha_{t}}{m} \sum_{i=1}^{m}L_{l}^{2}\left\|\bar{x}_{t}-x_{i, t}\right\|^{2}+\frac{2\alpha_{t}}{m} \sum_{i=1}^{m}\left\|B_{i, t}\right\|^{2}\right.\\
    &\left.+\frac{2 \alpha_{t}}{m} \sum_{i=1}^{m}L_{f}^{2}\left\| y_{i, t}^{*}-y_{i, t}\right\|^{2}+2 \alpha_{t}\left\|\frac{1}{m} \sum_{i=1}^{m} \bar{\nabla} f_{i}\left(x_{i, t}, y_{i, t}\right)+\frac{1}{m} \sum_{i=1}^{m} B_{i, t}-\bar{u}_{t}\right\|^{2} \right]
\end{align*}
where (a), (e) and (g) use the Lipschitz continuous gradients of $l$ (see Lemma~\ref{lemma_Lip}). (b) follows from the update rule of Algorithm~\ref{alg}. (c), (d) and (f) are because of $\left\| x+y \right\|^{2}\le 2\left\| x \right\|^{2}+2\left\| y \right\|^{2}, \forall x,y$.
\begin{align*}
    &2 \alpha_{t}\left\|\frac{1}{m} \sum_{i=1}^{m} \bar{\nabla} f_{i}\left(x_{i, t}, y_{i, t}\right)+\frac{1}{m} \sum_{i=1}^{m} B_{i, t}-\bar{u}_{t}\right\|^{2}=2 \alpha_{t}\left\|\frac{1}{m} \sum_{i=1}^{m} \bar{\nabla} f_{i}\left(x_{i, t}, y_{i, t}\right)+\frac{1}{m} \sum_{i=1}^{m} B_{i, t}-\bar{p}_{t}\right\|^{2}\\
    &=2 \alpha_{t}\left\|\frac{1}{m} \sum_{i=1}^{m} \bar{\nabla} f_{i}\left(x_{i, t}, y_{i, t}\right)+\frac{1}{m} \sum_{i=1}^{m} B_{i, t}-\frac{1}{m} \sum_{i=1}^{m} p_{i, t}\right\|^{2} \leq \frac{2 \alpha_{t}}{m} \sum_{i=1}^{m}\left\| \bar{\nabla} f_{i}\left(x_{i, t}, y_{i, t}\right)+B_{i, t}-p_{i, t}\right\|^{2}\\
    &\stackrel{(a)}{=} \frac{2 \alpha_{t}}{m} \sum_{i=1}^{m}\left\| e_{i,t}^{f}\right\|^{2}
\end{align*}
where (a) follow from the definition of $e_{i,t}^{f}$, which is $e_{i, t}^{f}:=p_{i}\left( x_{i,t},y_{i,t} \right)-\bar{\nabla} f_{i}\left( x_{i,t},y_{i,t} \right)-B_{i}\left( x_{i,t},y_{i,t} \right)$. Combine the above results, and the proof is completed.
\end{proof}

\subsection{Step 2: Error bound on $y^{*}(x)$}

\begin{lemma}
    Under Assumptions~\ref{asmp_up} and \ref{asmp_lo}, with $e_{i, t}^{g}$ defined as $e_{i, t}^{g}:=v_{i,t}-\nabla _{y} g_{i}\left( x_{i,t},y_{i,t} \right)$, the following inequality holds for Algorithm~\ref{alg}:
    \begin{equation*}
        \begin{aligned}
            \mathbb{E}\left[\left\|y_{i, t+1}-y_{i, t+1}^{*}\right\|^{2}\right] \le 
            &\mathbb{E}\left[\left(1+c_{1}\right)\left(1+c_{0}\right)\left(1-2 \beta_{t} \frac{\mu_{g} L_{g}}{\mu_{g}+L_{g}}\right)\left\|y_{i, t}-y_{i, t}^{*}\right\|^{2}\right. \\
            &\left.+\left(1+c_{1}\right)\left(1+c_{0}\right)\left(\beta_{t}^{2}-2 \beta_{t} \frac{1}{\mu_{g}+L_{g}}\right)\left\|\nabla_{y} g_{i}\left(x_{i, t}, y_{i, t}\right)\right\|^{2}\right. \\
            &\left.+\left(1+c_{1}\right)\left(1+\frac{1}{c_{0}}\right) \beta_{t}^{2}\left\|e_{i, t}^{g}\right\|^{2}\right. \\
            &\left.+2\left(1+\frac{1}{c_{1}}\right) L_{y}^{2} \alpha_{t}^{2}\left(\left\|u_{i, t}-\bar{u}_{t}\right\|^{2}+\left\|\bar{u}_{t}\right\|^{2}\right)\right]
        \end{aligned}
    \end{equation*}
    for all $t\in \left\{ 0,1,\ldots,T-1  \right\}$ with some arbitrary constants $c_{0},c_{1}> 0$, where the expectation is w.r.t. the stochasticity of the algorithm.
\end{lemma}

\begin{proof}
\begin{align*}
    \mathbb{E}\left[ \left\|y_{i, t+1}-y_{i, t+1}^{*}\right\|^{2} \right] &=\mathbb{E}\left[ \left\|y_{i, t+1}-y_{i, t}^{*}+y_{i, t}^{*}-y_{i, t+1}^{*}\right\|^{2} \right] \\
    & \stackrel{(a)}{\leq}\mathbb{E}\left[ \left(1+c_{1}\right)\left\|y_{i, t+1}-y_{i, t}^{*}\right\|^{2}+\left(1+\frac{1}{c_{1}}\right)\left\|y_{i, t}^{*}-y_{i, t+1}^{*}\right\|^{2} \right]\\
    &\stackrel{(b)}{\leq}\mathbb{E}\left[ \left(1+c_{1}\right) \left\| y_{i, t}-\beta_{t} v_{i, t}-y_{i, t}^{*} \right\|^{2}+\left(1+\frac{1}{c_{1}}\right) L_{y}^{2} \left\| x_{i, t}-x_{i, t+1} \right\|^{2} \right]\\
    &\stackrel{(c)}{\leq}\mathbb{E}\left[ \left(1+c_{1}\right) \left\| y_{i, t}-\beta_{t} v_{i, t}-y_{i, t}^{*} \right\|^{2}+2\left(1+\frac{1}{c_{1}}\right) L_{y}^{2}\alpha_{t}^{2} \left( \left\| u_{i, t}-\bar{u}_{t} \right\|^{2}+\left\| \bar{u}_{t} \right\|^{2} \right) \right]\\
    &=\mathbb{E}\left[ \left(1+c_{1}\right) \left\| y_{i, t}-\beta_{t}\nabla _{y}g_{i}\left( x_{i,t},y_{i,t} \right)+\beta_{t}\nabla _{y}g_{i}\left( x_{i,t},y_{i,t} \right)-\beta_{t} v_{i, t}-y_{i, t}^{*} \right\|^{2}\right.\\
    &\left.+2\left(1+\frac{1}{c_{1}}\right) L_{y}^{2}\alpha_{t}^{2} \left( \left\| u_{i, t}-\bar{u}_{t} \right\|^{2}+\left\| \bar{u}_{t} \right\|^{2} \right) \right]\\
    &\stackrel{(d)}{\leq}\mathbb{E}\left[ \left(1+c_{1}\right)\left( 1+c_{0} \right) \left\| y_{i, t}-\beta_{t}\nabla _{y}g_{i}\left( x_{i,t},y_{i,t} \right)-y_{i, t}^{*} \right\|^{2}\right.\\
    &\left.+\left(1+c_{1}\right)\left( 1+\frac{1}{c_{0}} \right)\beta_{t}^{2}\left\| \nabla _{y}g_{i}\left( x_{i,t},y_{i,t} \right)- v_{i, t}\right\|^{2}\right.\\
    &\left.+2\left(1+\frac{1}{c_{1}}\right) L_{y}^{2}\alpha_{t}^{2} \left( \left\| u_{i, t}-\bar{u}_{t} \right\|^{2}+\left\| \bar{u}_{t} \right\|^{2} \right) \right]
\end{align*}
where (a) and (d) result from Young's inequality. (b) is because of the update rule of Algorithm~\ref{alg} and the Lipschitzness of $y^{*}\left( \cdot  \right)$ (see Lemma~\ref{lemma_Lip}). (c) follows from the update rule of Algorithm~\ref{alg} and $\left\| x+y \right\|^{2}\le 2\left\| x \right\|^{2}+2\left\| y \right\|^{2}, \forall x,y$. To bound the first term on the right, we have 
\begin{align*}
    &\mathbb{E}\left[ \left\| y_{i, t}-\beta_{t}\nabla _{y}g_{i}\left( x_{i,t},y_{i,t} \right)-y_{i, t}^{*} \right\|^{2} \right]\\
    &=\mathbb{E}\left[ \left\|y_{i, t}-y_{i, t}^{*}\right\|^{2}+\beta_{t}^{2}\left\|\nabla_{y} g_{i}\left(x_{i, t}, y_{i, t}\right)\right\|^{2}-2 \beta_{t}\left\langle \nabla_{y} g_{i}\left(x_{i, t}, y_{i, t}\right), y_{i, t}-y_{i, t}^{*} \right\rangle \right]\\
    &\stackrel{(a)}{\leq}\mathbb{E}\left[ \left(1-2 \beta_{t} \frac{\mu_{g} L_{g}}{\mu_{g}+L_{g}}\right)\left\|y_{i, t}-y_{i, t}^{*}\right\|^{2}+\left(\beta_{t}^{2}-2 \beta_{t} \frac{1}{\mu_{g}+L_{g}}\right)\left\|\nabla_{y} g_{i}\left(x_{i, t}, y_{i, t}\right)\right\|^{2} \right]
\end{align*}
where (a) is due to $\mu_{g}$-strongly convexity and $L_{g}$-smoothness of the lower-level function $g_{i}\left( x_{i,t},y_{i,t} \right)$. Thus,
\begin{align*}
    \mathbb{E}\left[ \left\|y_{i, t+1}-y_{i, t+1}^{*}\right\|^{2} \right]& \leq\mathbb{E}\left[ \left(1+c_{1}\right)\left(1+c_{0}\right)\left(1-2 \beta_{t} \frac{\mu_{g} L_{g}}{\mu_{g}+L_{g}}\right)\left\|y_{i, t}-y_{i, t}^{*}\right\|^{2} \right.\\
    &\left.+\left(1+c_{1}\right)\left(1+c_{0}\right)\left(\beta_{t}^{2}-2 \beta_{t} \frac{1}{\mu_{g}+L_{g}}\right)\left\|\nabla_{y} g_{i}\left(x_{i, t}, y_{i,t}\right)\right\|^{2} \right.\\
    &\left.+\left(1+c_{1}\right)\left(1+\frac{1}{c_{0}}\right) \beta_{t}^{2}\left\|\nabla_{y} g_{i}\left(x_{i, t}, y_{i, t}\right)-v_{i, t}\right\|^{2} \right.\\
    &\left.+2\left(1+\frac{1}{c_{1}}\right) L_{y}^{2} \alpha_{t}^{2}\left(\left\|u_{i, t}-\bar{u}_{t}\right\|^{2}+\left\|\bar{u}_{t}\right\|^{2}\right) \right]\\
    &\stackrel{(a)}{=}\mathbb{E}\left[ \left(1+c_{1}\right)\left(1+c_{0}\right)\left(1-2 \beta_{t} \frac{\mu_{g} L_{g}}{\mu_{g}+L_{g}}\right)\left\|y_{i, t}-y_{i, t}^{*}\right\|^{2} \right.\\
    &\left.+\left(1+c_{1}\right)\left(1+c_{0}\right)\left(\beta_{t}^{2}-2 \beta_{t} \frac{1}{\mu_{g}+L_{g}}\right)\left\|\nabla_{y} g_{i}\left(x_{i, t}, y_{i,t}\right)\right\|^{2} \right.\\
    &\left.+\left(1+c_{1}\right)\left(1+\frac{1}{c_{0}}\right) \beta_{t}^{2}\left\|e_{i,t}^{g}\right\|^{2} \right.\\
    &\left.+2\left(1+\frac{1}{c_{1}}\right) L_{y}^{2} \alpha_{t}^{2}\left(\left\|u_{i, t}-\bar{u}_{t}\right\|^{2}+\left\|\bar{u}_{t}\right\|^{2}\right) \right]\\
\end{align*}
where (a) uses the definition of $e_{i,t}^{g}$, which is $e_{i,t}^{g}=v_{i, t}-\nabla_{y} g_{i}\left(x_{i, t}, y_{i, t}\right)$. Hence, the lemma is proved.
\end{proof}

\subsection{Step 3: Descent in the gradient estimation error of the upper-level function}

\begin{lemma}
    Define the gradient estimation error of the upper-level function as $e_{i, t}^{f}:=p_{i}\left( x_{i,t},y_{i,t} \right)-\bar{\nabla} f_{i}\left( x_{i,t},y_{i,t} \right)-B_{i}\left( x_{i,t},y_{i,t} \right)$. Under Assumptions~\ref{asmp_up}-\ref{asmp_sg}, Algorithm~\ref{alg} satisfies the following inequality:
    \begin{equation*}
        \begin{aligned}
            \mathbb{E}\left[\left\|e_{i, t+1}^{f}\right\|^{2}\right]\le 
            & \mathbb{E}\left[5 \eta^{2}\left\|e_{i, t}^{f}\right\|^{2}+5(1-\eta)^{2} \sigma_{f}^{2}+5 \eta^{2}\left\|B_{i, t+1}\right\|^{2}+5 \eta^{2}\left\|B_{i, t}\right\|^{2} \right.\\
            & \left. +5 \eta^{2} L_{f^{\prime}}^{2} \alpha_{t}^{2}\left\|u_{i, t}\right\|^{2}\right]
        \end{aligned}
    \end{equation*}
    for all $t\in \left\{ 0,1,\ldots,T-1  \right\}$, where the expectation is w.r.t. the stochasticity of the algorithm.
\end{lemma}

\begin{proof}
\begin{align*}
    \mathbb{E}\left[ \left\|e_{i, t+1}^{f}\right\|^{2} \right] &=\mathbb{E}\left[ \left\|p_{i, t+1}-\bar{\nabla} f_{i}\left(x_{i, t+1}, y_{i, t+1}\right)-B_{i, t+1}\right\|^{2} \right] \\
    & \stackrel{(a)}{=}\mathbb{E}\left[ \left\|\eta p_{i, t}+\left(1-\eta\right) \hat{\nabla} f_{i}\left(x_{i, t+1}, y_{i, t+1};\bar{\xi}_{i}\right)-\bar{\nabla} f_{i}\left(x_{i, t+1}, y_{i, t+1}\right)-B_{i, t+1}\right\|^{2} \right]\\
    &=\mathbb{E}\left[ \left\| \eta\left(p_{i, t}-\bar{\nabla} f_{i}\left(x_{i, t}, y_{i, t}\right)-B_{i, t}\right)\right.\right.\\
    &\left.+(1-\eta)\left(\hat{\nabla} f_{i}\left(x_{i, t+1}, y_{i, t+1};\bar{\xi}_{i}\right)-\bar{\nabla} f_{i}\left(x_{i, t+1}, y_{i, t+1}\right)-B_{i, t+1}\right)\right.\\
    &\left.\left.-\eta\left(\bar{\nabla} f_{i}\left(x_{i, t+1}, y_{i, t+1}\right)-\bar{\nabla} f_{i}\left(x_{i, t}, y_{i, t}\right)\right)+\eta B_{i, t}-\eta B_{i, t+1} \right\|^{2}\right]\\
    &\stackrel{(b)}{=}\mathbb{E}\left[ \left\| \eta e_{i, t}^{f} +(1-\eta)\left(\hat{\nabla} f_{i}\left(x_{i, t+1}, y_{i, t+1};\bar{\xi}_{i}\right)-\bar{\nabla} f_{i}\left(x_{i, t+1}, y_{i, t+1}\right)-B_{i, t+1}\right)\right.\right.\\
    &\left.\left.-\eta\left(\bar{\nabla} f_{i}\left(x_{i, t+1}, y_{i, t+1}\right)-\bar{\nabla} f_{i}\left(x_{i, t}, y_{i, t}\right)\right)+\eta B_{i, t}-\eta B_{i, t+1} \right\|^{2}\right]\\
    &\stackrel{(c)}{\leq}\mathbb{E}\left[  5 \eta^{2}\left\|e_{i, t}^{f}\right\|^{2}+5(1-\eta)^{2}\left\|\hat{\nabla} f_{i}\left(x_{i, t+1}, y_{i, t+1};\bar{\xi}_{i}\right)-\bar{\nabla} f_{i}\left(x_{i, t+1,} y_{i, t+1}\right)-B_{i, t+1}\right\|^{2}\right. \\
    &\left.+5 \eta^{2}\left\|\bar{\nabla} f_{i}\left(x_{i, t+1}, y_{i, t+1}\right)-\bar{\nabla} f_{i}\left(x_{i, t}, y_{i, t}\right)\right\|^{2}+5 \eta^{2}\left\|B_{i, t+1}\right\|^{2}+5 \eta^{2}\left\|B_{i, t}\right\|^{2}\right]\\
    &\stackrel{(d)}{\leq}\mathbb{E}\left[  5 \eta^{2}\left\|e_{i, t}^{f}\right\|^{2}+5(1-\eta)^{2}\sigma_{f}^{2}+5 \eta^{2}\left\|\bar{\nabla} f_{i}\left(x_{i, t+1}, y_{i, t+1}\right)-\bar{\nabla} f_{i}\left(x_{i, t}, y_{i, t}\right)\right\|^{2}\right.\\
    &\left.+5 \eta^{2}\left\|B_{i, t+1}\right\|^{2}+5 \eta^{2}\left\|B_{i, t}\right\|^{2}\right]\\
    &\stackrel{(e)}{\leq}\mathbb{E}\left[  5 \eta^{2}\left\|e_{i, t}^{f}\right\|^{2}+5(1-\eta)^{2}\sigma_{f}^{2}+5 \eta^{2}L_{f^{'}}^{2}\left\|x_{i,t+1}-x_{i,t}\right\|^{2}+5 \eta^{2}\left\|B_{i, t+1}\right\|^{2}+5 \eta^{2}\left\|B_{i, t}\right\|^{2}\right]\\
    &\stackrel{(f)}{=}\mathbb{E}\left[  5 \eta^{2}\left\|e_{i, t}^{f}\right\|^{2}+5(1-\eta)^{2}\sigma_{f}^{2}+5 \eta^{2}L_{f^{'}}^{2}\alpha_{t}^{2}\left\|u_{i,t}\right\|^{2}+5 \eta^{2}\left\|B_{i, t+1}\right\|^{2}+5 \eta^{2}\left\|B_{i, t}\right\|^{2}\right]
\end{align*}
where (a) follows from the update rule of $p_{i}\left( x_{i,t},y_{i,t} \right)$. (b) uses the definition of $e_{i, t}^{f}$. (c) is due to $\left\| z_{1}+\cdots +z_{k} \right\|^{2}\le k\left\| z_{1} \right\|^{2}+\cdots +k\left\| z_{k} \right\|^{2}$. (d) uses Assumption~\ref{asmp_sg}.1. (e) is because of the  Lipschitzness in Lemma~\ref{lemma_Lip}. (f) uses the update rule of $x_{i,t}$. 
\end{proof}

\subsection{Step 4: Descent in the gradient estimation error of the lower-level function}

\begin{lemma}
    Define the gradient estimation error of the lower-level function as $e_{i, t}^{g}:=v_{i,t}-\nabla _{y} g_{i}\left( x_{i,t},y_{i,t} \right)$. Under Assumptions~\ref{asmp_up}-\ref{asmp_sg}, Algorithm~\ref{alg} satisfies the following inequality:
    \begin{equation*}
        \begin{aligned}
            \mathbb{E}\left[\left\|e_{i, t+1}^{g}\right\|^{2}\right] \le &\mathbb{E}\left[\left(3 \gamma^{2}+12 \gamma^{2} L_{g_{y}}^{2} \beta_{t}^{2}\right)\left\|e_{i, t}^{g}\right\|^{2}+3(1-\gamma)^{2} \sigma_{g}^{2}+6 \gamma^{2} L_{g}^{2} \alpha_{t}^{2}\left\|u_{i, t}\right\|^{2}\right. \\
            &\left. +12 \gamma^{2} L_{g_{y}}^{2} \beta_{t}^{2}\left\|\nabla_{y} g_{i}\left(x_{i t}, y_{i, t}\right)\right\|^{2}\right]
        \end{aligned}
    \end{equation*}
    for all $t\in \left\{ 0,1,\ldots,T-1  \right\}$, where the expectation is w.r.t. the stochasticity of the algorithm.
\end{lemma}

\begin{proof}
\begin{align*}
    \mathbb{E}\left[ \left\|e_{i, t+1}^{g}\right\|^{2}\right] &=\mathbb{E}\left[ \left\|v_{i, t+1}-\nabla_{y} g_{i}\left(x_{i, t+1}, y_{i, t+1}\right)\right\|^{2}\right] \\
    & \stackrel{(a)}{=}\mathbb{E}\left[ \left\|\gamma v_{i, t}+\left(1-\gamma\right) \nabla_{y} g_{i}\left(x_{i, t+1}, y_{i, t+1};\zeta_{i}\right)-\nabla_{y} g_{i}\left(x_{i, t+1}, y_{i, t+1}\right)\right\|^{2}\right]\\
    &\stackrel{(b)}{=}\mathbb{E}\left[  \| \gamma e_{i, t}^{g}+(1-\gamma)\left(\nabla _{y} g_{i}\left(x_{i, t+1}, y_{i, t+1};\zeta_{i}\right)-\nabla_{y} g_{i}\left(x_{i, t+1}, y_{i, t+1}\right)\right)\right. \\
    &\left.-\gamma\left(\nabla_{y} g_{i}\left(x_{i, t+1}, y_{i, t+1}\right)-\nabla_{y} g_{i}\left(x_{i, t}, y_{i, t}\right)\right) \|^{2}\right]\\
    &\stackrel{(c)}{\le }\mathbb{E}\left[  3\gamma^{2}\|  e_{i, t}^{g}\|^{2}+3(1-\gamma)^{2}\|\nabla _{y} g_{i}\left(x_{i, t+1}, y_{i, t+1};\zeta_{i}\right)-\nabla_{y} g_{i}\left(x_{i, t+1}, y_{i, t+1}\right)\|^{2}\right. \\
    &\left.+3\gamma^{2}\|\nabla_{y} g_{i}\left(x_{i, t+1}, y_{i, t+1}\right)-\nabla_{y} g_{i}\left(x_{i, t}, y_{i, t}\right) \|^{2}\right]\\
    &\stackrel{(d)}{\le }\mathbb{E}\left[  3\gamma^{2}\|  e_{i, t}^{g}\|^{2}+3(1-\gamma)^{2}\sigma_{g}^{2}+3\gamma^{2}\|\nabla_{y} g_{i}\left(x_{i, t+1}, y_{i, t+1}\right)-\nabla_{y} g_{i}\left(x_{i, t}, y_{i, t}\right) \|^{2}\right]\\
    &\le\mathbb{E}\left[  3\gamma^{2}\|  e_{i, t}^{g}\|^{2}+3(1-\gamma)^{2}\sigma_{g}^{2}+6\gamma^{2}\|\nabla_{y} g_{i}\left(x_{i, t+1}, y_{i, t+1}\right)-\nabla_{y} g_{i}\left(x_{i, t+1}, y_{i, t}\right)\|^{2}\right.\\
    &\left.+6\gamma^{2}\|\nabla_{y} g_{i}\left(x_{i, t+1}, y_{i, t}\right)-\nabla_{y} g_{i}\left(x_{i, t}, y_{i, t}\right) \|^{2}\right]\\
    &\stackrel{(e)}{\le } 3\gamma^{2}\|  e_{i, t}^{g}\|^{2}+3(1-\gamma)^{2}\sigma_{g}^{2}+6\gamma^{2}L_{g}^{2}\|x_{i,t+1}-x_{i,t}\|^{2}+6\gamma^{2}L_{g_{y}}^{2}\|y_{i,t+1}-y_{i,t} \|^{2}\\
    &\stackrel{(f)}{\le }\mathbb{E}\left[  3\gamma^{2}\|  e_{i, t}^{g}\|^{2}+3(1-\gamma)^{2}\sigma_{g}^{2}+6\gamma^{2}L_{g}^{2}\alpha_{t}^{2}\|u_{i,t}\|^{2}+6\gamma^{2}L_{g_{y}}^{2}\beta_{t}^{2}\|v_{i,t} \|^{2} \right]\\
    &\stackrel{(g)}{=}\mathbb{E}\left[  3\gamma^{2}\|  e_{i, t}^{g}\|^{2}+3(1-\gamma)^{2}\sigma_{g}^{2}+6\gamma^{2}L_{g}^{2}\alpha_{t}^{2}\|u_{i,t}\|^{2}+6\gamma^{2}L_{g_{y}}^{2}\beta_{t}^{2}\|e_{i,t}^{g}+\nabla _{y}g_{i}\left( x_{i,t},y_{i,t} \right) \|^{2} \right]\\
    &\stackrel{(h)}{\le }\mathbb{E}\left[  \left( 3\gamma^{2}+12\gamma^{2}L_{g_{y}}^{2}\beta_{t}^{2} \right)\|  e_{i, t}^{g}\|^{2}+3(1-\gamma)^{2}\sigma_{g}^{2}+6\gamma^{2}L_{g}^{2}\alpha_{t}^{2}\|u_{i,t}\|^{2} \right.\\
    &\left.+12\gamma^{2}L_{g_{y}}^{2}\beta_{t}^{2}\|\nabla _{y}g_{i}\left( x_{i,t},y_{i,t} \right) \|^{2} \right]
\end{align*}
where (a) follows from the update rule of $v_{i,t}$. (b) and (g) use the definition of $e_{i, t}^{g}$. (c) is due to $\left\| z_{1}+\cdots +z_{k} \right\|^{2}\le k\left\| z_{1} \right\|^{2}+\cdots +k\left\| z_{k} \right\|^{2}$. (d) uses Assumption~\ref{asmp_sg}.2. (e) is because of Assumption~\ref{asmp_lo}.2. (f) uses the update rules. (h) is due to $\left\| x+y \right\|^{2}\le 2\left\| x \right\|^{2}+2\left\| y \right\|^{2}$.
\end{proof}

\subsection{Step 5: Iterates Contraction}

\begin{lemma}
    The following contraction properties of the iterates hold:
    \begin{equation*}
        \left\|x_{t}-1 \otimes \bar{x}_{t}\right\|^{2}\le \left(1+c_{2}\right) \lambda^{2}\left\|x_{t-1}-1 \otimes \bar{x}_{t-1}\right\|^{2}+\left(1+\frac{1}{c_{2}}\right) \alpha_{t-1}^{2}\left\|u_{t-1}-1 \otimes \bar{u}_{t-1}\right\|^{2}
    \end{equation*}
    \begin{equation*}
        \left\|u_{t}-1 \otimes \bar{u}_{t}\right\|^{2}\le \left(1+c_{3}\right) \lambda^{2}\left\|u_{t-1}-1 \otimes \bar{u}_{t-1}\right\|^{2}+\left(1+\frac{1}{c_{3}}\right)\left\|p_{t}-p_{t-1}\right\|^{2}
    \end{equation*}
    where $c_{2},c_{3}> 0$ are some arbitrary constants. In addition, we have
    \begin{equation*}
        \mathbb{E}\left[ \left\| p_{t}-p_{t-1} \right\|^{2} \right]\le \mathbb{E}\left[ 3 m(1-\eta)^{2} \sigma_{f}^{2}+3 m(1-\eta)^{2} C_{f}^{2}+3(1-\eta)^{2} \sum_{i=1}^{m}\left\|B_{i,t}\right\|^{2} \right]
    \end{equation*}
    where the expectation is w.r.t. the stochasticity of the algorithm.
\end{lemma}

\begin{proof}
Define $\tilde{\mathrm{M}}=\mathrm{M} \otimes \mathrm{I}_{m}$. For the iterates $x_{t}$, we have
\begin{equation*}
    \left\|\tilde{\mathrm{M}} x_{t}-1 \otimes \bar{x}_{t}\right\|^{2}=\left\|\tilde{\mathrm{M}}\left(x_{t}-1 \otimes \bar{x}_{t}\right)\right\|^{2} \leq \lambda^{2}\left\|x_{t}-1 \otimes \bar{x}_{t}\right\|^{2}
\end{equation*}
This is because $x_{t}-1 \otimes x_{t}$ is is orthogonal to $1$, which is the eigenvector corresponding to the largest eigenvalue of $\tilde{\mathrm{M}}$, and $\lambda=\max\left\{ \left| \lambda_{2} \right|,\left| \lambda_{m} \right| \right\}$. Recall that $\bar{x}_{t}=\bar{x}_{t-1}-\alpha_{t-1} \bar{u}_{t-1}$, hence,
\begin{align*}
    \left\|x_{t}-1 \otimes \bar{x}_{t}\right\|^{2} &=\left\|\tilde{\mathrm{M}} x_{t-1}-\alpha_{t-1} u_{t-1}-1 \otimes\left(\bar{x}_{t-1}-\alpha_{t-1} \bar{u}_{t-1}\right)\right\|^{2} \\
    & \leq\left(1+c_{2}\right)\left\|\tilde{\mathrm{M}} x_{t-1}-1 \otimes \bar{x}_{t-1}\right\|^{2}+\left(1+\frac{1}{c_{2}}\right) \alpha_{t-1}^{2}\left\|u_{t-1}-1 \otimes \bar{u}_{t-1}\right\|^{2} \\
    & \leq\left(1+c_{2}\right) \lambda^{2}\left\|x_{t-1}-1 \otimes \bar{x}_{t-1}\right\|^{2}+\left(1+\frac{1}{c_{2}}\right) \alpha_{t-1}^{2}\left\|u_{t-1}-1 \otimes \bar{u}_{t-1}\right\|^{2}
\end{align*}
For $u_{t}$, we have 
\begin{align*}
    \left\|u_{t}-1 \otimes \bar{u}_{t}\right\|^{2}&=\left\|\tilde{\mathrm{M}} u_{t-1}+p_{t}-p_{t-1}-1 \otimes\left(\bar{u}_{t-1}+\bar{p}_{t}-\bar{p}_{t-1}\right)\right\|^{2}\\
    &\leq\left(1+c_{3}\right)\left\|\tilde{\mathrm{M}} u_{t-1}-1 \otimes \bar{u}_{t-1}\right\|^{2}+\left(1+\frac{1}{c_{3}}\right) \| p_{t}-p_{t-1}-1 \otimes\left(\bar{p}_{t}-\bar{p}_{t-1}\right) \|^{2}\\
    &\leq\left(1+c_{3}\right) \lambda^{2}\left\|u_{t-1}-1 \otimes \bar{u}_{t-1}\right\|^{2}+\left(1+\frac{1}{c_{3}}\right) \| p_{t}-p_{t-1}-1 \otimes\left(\bar{p}_{t}-\bar{p}_{t-1}\right) \|^{2}\\
    &\leq\left(1+c_{3}\right) \lambda^{2}\left\|u_{t-1}-1 \otimes \bar{u}_{t-1}\right\|^{2}+\left(1+\frac{1}{c_{3}}\right)\left\|\left(\mathrm{I}-\frac{1}{m}\left(11^{\top}\right) \otimes \mathrm{I}\right)\left(p_{t}-p_{t-1}\right)\right\|^{2}\\
    &\stackrel{(a)}{\leq}\left(1+c_{3}\right) \lambda^{2}\left\|u_{t-1}-1 \otimes \bar{u}_{t-1}\right\|^{2}+\left(1+\frac{1}{c_{3}}\right)\left\|p_{t}-p_{t-1}\right\|^{2}
\end{align*}
where (a) is because of $\left\| \mathrm{I}-\frac{1}{m}\left(11^{\top}\right) \otimes \mathrm{I} \right\|\le 1$.

According to the update of $p_{i}\left( x_{i,t},y_{i,t} \right)$, we have
\begin{align*}
    \mathbb{E}\left[ \left\|p_{t}-p_{t-1}\right\|^{2}\right] &=\mathbb{E}\left[ \sum_{i=1}^{m}\left\|p_{i, t}-p_{i, t-1}\right\|^{2} \right] \\
    & \stackrel{(a)}{=}\mathbb{E}\left[  \sum_{i=1}^{m}\left\|(1-\eta) \hat{\nabla} f_{i}\left(x_{i, t}, y_{i, t};\bar{\xi}_{i}\right)\right\|^{2} \right]\\
    &=\mathbb{E}\left[ \sum_{i=1}^{m}(1-\eta)^{2} \| \hat{\nabla} f_{i}\left(x_{i, t}, y_{i, t};\bar{\xi}_{i}\right)-\bar{\nabla} f_{i}\left(x_{i, t}, y_{i, t}\right)-B_{i, t}+\bar{\nabla} f_{i}\left(x_{i, t}, y_{i, t}\right)+B_{i, t} \|^{2} \right]\\
    &\stackrel{(b)}{\le }\mathbb{E}\left[ \sum_{i=1}^{m}3(1-\eta)^{2}\left\|\hat{\nabla} f_{i}\left(x_{i, t}, y_{i, t};\bar{\xi}_{i}\right)-\bar{\nabla} f_{i}\left(x_{i, t}, y_{i, t}\right)-B_{i, t}\right\|^{2} \right. \\
    & \left.+\sum_{i=1}^{m}3(1-\eta)^{2}\left\| \bar{\nabla} f_{i}\left( x_{i t}, y_{i, t} \right) \right\|^{2}+\sum_{i=1}^{m}3(1-\eta)^{2}\left\| B_{i, t} \right\|^{2} \right]\\
    &\stackrel{(c)}{\le }\mathbb{E}\left[ 3m(1-\eta)^{2}\sigma_{f}^{2}+3m(1-\eta)^{2}C_{f}^{2}+\sum_{i=1}^{m}3(1-\eta)^{2}\left\| B_{i, t} \right\|^{2} \right]
\end{align*}
where (a) is due to $p_{i,t}=\eta^{t}p_{i,0}+\left( 1-\eta \right)\sum_{j=0}^{t}\eta^{t-j}\hat{\nabla} f_{i}\left( x_{i,t},y_{i,t};\bar{\xi}_{i} \right)$ and $p_{i,0}=0$. (b) uses $\left\| z_{1}+\cdots +z_{k} \right\|^{2}\le k\left\| z_{1} \right\|^{2}+\cdots +k\left\| z_{k} \right\|^{2}$. (c) is because of Assumption~\ref{asmp_up}.4 and \ref{asmp_sg}.1.
\end{proof}

\subsection{Step 6: Descent in the potential function}
Define the potential function $W_{t}$ as:
\begin{equation*}
    W_{t}=l\left(\bar{x}_{t}\right)+\left\|y_{t}-y_{t}^{*}\right\|^{2}+\alpha_{t-1}\left\|e_{t}^{f}\right\|^{2}+\alpha_{t-1}\left\|e_{t}^{g}\right\|^{2}+\left\|x_{t}-1 \otimes \bar{x}_{t}\right\|^{2}+\alpha_{t-1}\left\|u_{t}-1 \otimes \bar{u}_{t}\right\|^{2}
\end{equation*}

\begin{lemma}
    Denote  $L_{\mu_{g}}=\frac{\mu_{g} L_{g}}{\mu_{g}+L_{g}}$ and $B=\frac{C_{g_{x y}} C_{f_{y}}}{\mu_{g}}\left(1-\frac{\mu_{g}}{L_{g}}\right)^{K}$. Choose $c_{0}=\frac{\beta_{t} L_{\mu_{g}}}{1-2 \beta_{t} L_{\mu_{g}}}$ and $c_{1}=\frac{\beta_{t} L_{\mu_{g}}}{2\left( 1- \beta_{t} L_{\mu_{g}} \right)}$. Then the iterates generated by Algorithm~\ref{alg} when the outer problem is smooth but possibly non-convex satisfy:
    \begin{align*}
        \mathbb{E}\left[ W_{t+1}-W_{t} \right]\leq &\mathbb{E}\left[ -\frac{\alpha_{t}}{2}\left\|\nabla l\left(\bar{x}_{t}\right)\right\|^{2}+\left(\frac{2 \alpha_{t}L_{f}^{2}}{m}-\frac{\beta_{t}L_{\mu_{g}}}{2} \right)\left\|y_{t}-y_{t}^{*}\right\|^{2}\right.\\
        &\left. + \left[ \frac{2\alpha_{t} L_{l}^{2}}{m}+\left( 1+c_{2} \right)\lambda^{2}-1 \right]\left\|x_{t}-1 \otimes \bar{x}_{t}\right\|^{2} \right.\\
        &\left. +\left[ \frac{4 L_{y}^{2} \alpha_{t}^{2}}{\beta_{t} L_{\mu_{g}}}+\left(1+\frac{1}{c_{2}}\right) \alpha_{t}^{2}+\left(1+c_{3}\right) \lambda^{2}\alpha_{t}-\alpha_{t-1} \right]\left\|u_{t}-1 \otimes \bar{u}_{t}\right\|^{2} \right.\\
        &\left. +\alpha_{t}\left[ 2B^{2}+5(1-\eta)^{2} m \sigma_{f}^{2}+3(1-\gamma)^{2} m \sigma_{g}^{2}+10\eta^{2}mB^{2} \right] \right.\\
        &\left. +\alpha_{t}\left(1+\frac{1}{c_{3}}\right)\left[3 m(1-\eta)^{2} \sigma_{f}^{2}+3 m(1-\eta)^{2} C_{f}^{2}+3(1-\eta)^{2} m B^{2}\right] \right]
    \end{align*}
    with the following conditions:
    \begin{align*}
        &\beta_{t}\le \frac{1}{\mu_{g}+L_{g}}\\
        &\left( 3 \gamma^{2}+12 \gamma^{2} L_{g_{y}}^{2} \beta_{t}^{2} \right)\alpha_{t}-\alpha_{t-1} \leq-\frac{2 \beta_{t}}{L_{\mu_{g}}}\\
        &5 \eta^{2}\alpha_{t}-\alpha_{t-1} \leq-\frac{2 \alpha_{t}}{m} \\
        &-\left(\frac{\alpha_{t}}{2}-\frac{L_{l} \alpha_{t}^{2}}{2}\right)+\frac{4 L_{y}^{2} \alpha_{t}^{2} m}{\beta_{t} L _{\mu_{g}}}+6 \gamma^{2} L_{g}^{2} \alpha_{t}^{3} m+5 \eta^{2} L_{f^{\prime}}^{2} \alpha_{t}^{3} m \leq 0 \\
        &12 \gamma^{2} L_{g_{y}}^{2} \beta_{t}^{2}\alpha_{t}-\frac{\beta_{t}}{\mu_{g}+L_{g}} \leq 0
    \end{align*}
\end{lemma}

\begin{proof}
From the results of Step 1, we have 
\begin{align*}
    \mathbb{E}\left[ l\left( \bar{x}_{t+1} \right)-l\left( \bar{x}_{t} \right)\right]&\le\mathbb{E}\left[  -\frac{\alpha_{t}}{2}\left\|\nabla l\left(\bar{x}_{t}\right)\right\|^{2}-\left(\frac{\alpha_{t}}{2}-\frac{L_{l} \alpha_{t}^{2}}{2}\right)\left\|\bar{u}_{t}\right\|^{2}+\frac{2\alpha_{t}}{m} \sum_{i=1}^{m} L_{l}^{2}\left\|\bar{x}_{t}-x_{i, t}\right\|^{2}\right. \\
    &\left.+\frac{2 \alpha_{t}}{m} \sum_{i=1}^{m}\left\|B_{i, t}\right\|^{2}+\frac{2 \alpha_{t}}{m} \sum_{i=1}^{m} L_{f}^{2}\left\|y_{i, t}^{*}-y_{i, t}\right\|^{2}+\frac{2 \alpha_{t}}{m} \sum_{i=1}^{m}\left\|e_{i, t}^{f}\right\|^{2}\right]\\
    &\le\mathbb{E}\left[  -\frac{\alpha_{t}}{2}\left\|\nabla l\left(\bar{x}_{t}\right)\right\|^{2}-\left(\frac{\alpha_{t}}{2}-\frac{L_{l} \alpha_{t}^{2}}{2}\right)\left\|\bar{u}_{t}\right\|^{2}+\frac{2\alpha_{t}}{m}  L_{l}^{2}\left\|x_{t}-1\otimes \bar{x}_{t}\right\|^{2}\right. \\
    &\left.+\frac{2 \alpha_{t}}{m} \sum_{i=1}^{m}\left\|B_{i, t}\right\|^{2}+\frac{2 \alpha_{t}}{m}  L_{f}^{2}\left\|y_{t}^{*}-y_{t}\right\|^{2}+\frac{2 \alpha_{t}}{m} \sum_{i=1}^{m}\left\|e_{i, t}^{f}\right\|^{2}\right]
\end{align*}

With the results from Step 2, we get
\begin{align*}
    \mathbb{E}\left[ \left\|y_{t+1}-y_{t+1}^{*}\right\|^{2}-\left\|y_{t}-y_{t}^{*}\right\|^{2}\right]&=\mathbb{E}\left[  \sum_{i=1}^{m}\left[\left\|y_{i, t+1}-y_{i, t+1}^{*}\right\|^{2}-\left\|y_{i, t}-y_{i, t}^{*}\right\|^{2}\right] \right]\\
    &\leq\mathbb{E}\left[  {\left[\left(1+c_{1}\right)\left(1+c_{0}\right)\left(1-2 \beta_{t} \frac{\mu_{g} L_{g}}{\mu_{g}+L_{g}}\right)-1\right]\left\|y_{t}-y_{t}^{*}\right\|^{2} } \right.\\
    &+\left(1+c_{1}\right)\left(1+\frac{1}{c_{0}}\right) \beta_{t}^{2} \sum_{i=1}^{m}\left\|e_{i, t}^{g}\right\|^{2} \\
    &+2\left(1+\frac{1}{c_{1}}\right) L_{y}^{2} \alpha_{t}^{2}\left(\left\|u_{t}-1 \otimes \bar{u}_{t}\right\|^{2}+m\left\|\bar{u}_{t}\right\|^{2}\right) \\
    &\left.+\left(1+c_{1}\right)\left(1+c_{0}\right)\left(\beta_{t}^{2}-2 \beta_{t} \frac{1}{\mu_{g}+L_{g}}\right) \sum_{i=1}^{m}\left\|\nabla_{y} g_{i}\left(x_{i, t}, y_{i, t}\right)\right\|^{2}\right]
\end{align*}
Denote $L_{\mu_{g}}=\frac{\mu_{g} L_{g}}{\mu_{g}+L_{g}}$. Choose $c_{0}$ and $c_{1}$ such that
\begin{equation*}
    \left(1+c_{1}\right)\left(1+c_{0}\right)\left(1-2 \beta_{t} L_{\mu_{g}}\right)=1-\frac{\beta_{t} L_{\mu_{g}}}{2}
\end{equation*}
Thus, 
\begin{equation*}
    c_{0}=\frac{\beta_{t} L_{\mu_{g}}}{1-2 \beta_{t} L_{\mu_{g}}},\quad c_{1}=\frac{\beta_{t} L_{\mu_{g}}}{2\left( 1-\beta_{t} L_{\mu_{g}} \right)}
\end{equation*}
Moreover, this implies that 
\begin{equation*}
    1+\frac{1}{c_{0}}=1+\frac{1-2 \beta_{t} L_{\mu_{g}}}{\beta_{t} L_{\mu_{g}}}\le \frac{1}{\beta_{t} L_{\mu_{g}}},\quad 1+\frac{1}{c_{1}}=\frac{2\left( 1-\beta_{t} L_{\mu_{g}} \right)}{\beta_{t} L_{\mu_{g}}}\le \frac{2}{\beta_{t} L_{\mu_{g}}}
\end{equation*}

Thus, we have
\begin{align*}
    \mathbb{E}\left[ \left\|y_{t+1}-y_{t+1}^{*}\right\|^{2}-\left\|y_{t}-y_{t}^{*}\right\|^{2}\right]& \mathbb{E}\left[ \leq {-\frac{\beta_{t}L_{\mu_{g}}}{2}\left\|y_{t}-y_{t}^{*}\right\|^{2} }+\frac{2}{\beta_{t}L_{\mu_{g}}} \beta_{t}^{2} \sum_{i=1}^{m}\left\|e_{i, t}^{g}\right\|^{2}\right. \\
    &+\frac{4L_{y}^{2} \alpha_{t}^{2}}{\beta_{t}L_{\mu_{g}}} \left(\left\|u_{t}-1 \otimes \bar{u}_{t}\right\|^{2}+m\left\|\bar{u}_{t}\right\|^{2}\right) \\
    &\left.-\left( \frac{2\beta_{t}}{\mu_{g}+L_{g}}-\beta_{t}^{2} \right) \sum_{i=1}^{m}\left\|\nabla_{y} g_{i}\left(x_{i, t}, y_{i, t}\right)\right\|^{2}\right]\\
    &\stackrel{(a)}{\le }\mathbb{E}\left[  {-\frac{\beta_{t}L_{\mu_{g}}}{2}\left\|y_{t}-y_{t}^{*}\right\|^{2} }+\frac{2}{\beta_{t}L_{\mu_{g}}} \beta_{t}^{2} \sum_{i=1}^{m}\left\|e_{i, t}^{g}\right\|^{2}\right. \\
    &+\frac{4L_{y}^{2} \alpha_{t}^{2}}{\beta_{t}L_{\mu_{g}}} \left(\left\|u_{t}-1 \otimes \bar{u}_{t}\right\|^{2}+m\left\|\bar{u}_{t}\right\|^{2}\right) \\
    &\left.-\frac{\beta_{t}}{\mu_{g}+L_{g}} \sum_{i=1}^{m}\left\|\nabla_{y} g_{i}\left(x_{i, t}, y_{i, t}\right)\right\|^{2}\right]
\end{align*}
where (a) choose $\beta_{t}\le \frac{1}{\mu_{g}+L_{g}}$.

With the results from Step 3 and 4, we have
\begin{align*}
    \mathbb{E}\left[ \alpha_{t}\left\|e_{i, t+1}^{f}\right\|^{2}-\alpha_{t-1}\left\|e_{i, t}^{f}\right\|^{2}\right]&\le\mathbb{E}\left[  \left( 5 \eta^{2}\alpha_{t}-\alpha_{t-1} \right)\left\|e_{i, t}^{f}\right\|^{2}+5(1-\eta)^{2}\sigma_{f}^{2}\alpha_{t}+5 \eta^{2}L_{f^{'}}^{2}\alpha_{t}^{3}\left\|u_{i,t}\right\|^{2}\right.\\
    &\left.+5 \eta^{2}\alpha_{t}\left\|B_{i, t+1}\right\|^{2}+5 \eta^{2}\alpha_{t}\left\|B_{i, t}\right\|^{2}\right]\\
    &\stackrel{(a)}{\le }\mathbb{E}\left[  -\frac{2\alpha_{t}}{m}\left\|e_{i, t}^{f}\right\|^{2}+5(1-\eta)^{2}\sigma_{f}^{2}\alpha_{t}+5 \eta^{2}L_{f^{'}}^{2}\alpha_{t}^{3}\left\|u_{i,t}\right\|^{2}\right.\\
    &\left.+5 \eta^{2}\alpha_{t}\left\|B_{i, t+1}\right\|^{2}+5 \eta^{2}\alpha_{t}\left\|B_{i, t}\right\|^{2}\right]
\end{align*}
where (a) choose $5 \eta^{2}\alpha_{t}-\alpha_{t-1}\le -\frac{2\alpha_{t}}{m}$.
\begin{align*}
    \mathbb{E}\left[ \alpha_{t}\left\|e_{i, t+1}^{g}\right\|^{2}-\alpha_{t-1}\left\|e_{i, t}^{g}\right\|^{2}\right] &\le  \mathbb{E}\left[ \left[ \left( 3\gamma^{2}+12\gamma^{2}L_{g_{y}}^{2}\beta_{t}^{2} \right)\alpha_{t}-\alpha_{t-1} \right]\|  e_{i, t}^{g}\|^{2}+3(1-\gamma)^{2}\sigma_{g}^{2}\alpha_{t}\right.\\
    &\left.+6\gamma^{2}L_{g}^{2}\alpha_{t}^{3}\|u_{i,t}\|^{2}+12\gamma^{2}L_{g_{y}}^{2}\beta_{t}^{2}\alpha_{t}\|\nabla _{y}g_{i}\left( x_{i,t},y_{i,t} \right) \|^{2}\right]\\
    &\stackrel{(a)}{\le }\mathbb{E}\left[   -\frac{2\beta_{t}}{L_{\mu_{g}}}\|  e_{i, t}^{g}\|^{2}+3(1-\gamma)^{2}\sigma_{g}^{2}\alpha_{t}+6\gamma^{2}L_{g}^{2}\alpha_{t}^{3}\|u_{i,t}\|^{2}\right.\\
    &\left.+12\gamma^{2}L_{g_{y}}^{2}\beta_{t}^{2}\alpha_{t}\|\nabla _{y}g_{i}\left( x_{i,t},y_{i,t} \right) \|^{2}\right]
\end{align*}
where (a) choose $\left( 3\gamma^{2}+12\gamma^{2}L_{g_{y}}^{2}\beta_{t}^{2} \right)\alpha_{t}-\alpha_{t-1} \le -\frac{2\beta_{t}}{L_{\mu_{g}}}$.

According to the result of step 5, we have
\begin{align*}
    \left\|x_{t}-1 \otimes \bar{x}_{t}\right\|^{2}-\left\|x_{t-1}-1 \otimes \bar{x}_{t-1}\right\|^{2}&\le \left( \left(1+c_{2}\right) \lambda^{2}-1 \right)\left\|x_{t-1}-1 \otimes \bar{x}_{t-1}\right\|^{2}\\
    &+\left(1+\frac{1}{c_{2}}\right) \alpha_{t-1}^{2}\left\|u_{t-1}-1 \otimes \bar{u}_{t-1}\right\|^{2}
\end{align*}
\begin{align*}
    \mathbb{E}\left[ \left\|u_{t}-1 \otimes \bar{u}_{t}\right\|^{2}\right]&\le\mathbb{E}\left[  \left(1+c_{3}\right) \lambda^{2}\left\|u_{t-1}-1 \otimes \bar{u}_{t-1}\right\|^{2}+\left(1+\frac{1}{c_{3}}\right)\left\|p_{t}-p_{t-1}\right\|^{2}\right]\\
    &\stackrel{(a)}{\le }\mathbb{E}\left[  \left(1+c_{3}\right) \lambda^{2}\left\|u_{t-1}-1 \otimes \bar{u}_{t-1}\right\|^{2}\right.\\
    &\left.+\left(1+\frac{1}{c_{3}}\right)\left[ 3 m(1-\eta)^{2} \sigma_{f}^{2}+3 m(1-\eta)^{2} C_{f}^{2}+3(1-\eta)^{2} mB^{2} \right]\right]\\
\end{align*}
where (a) follows from Lemma~\ref{lemma_B}, and denote $B=\frac{C_{g_{x y}} C_{f_{y}}}{\mu_{g}}\left(1-\frac{\mu_{g}}{L_{g}}\right)^{K}$. Then, we have
\begin{align*}
    \mathbb{E}\left[ \alpha_{t-1}\left\|u_{t}-1 \otimes \bar{u}_{t}\right\|^{2}-\alpha_{t-2}\right.&\left.\left\|u_{t-1}-1 \otimes \bar{u}_{t-1}\right\|^{2}\right]\le\mathbb{E}\left[  \left( \left(1+c_{3}\right) \lambda^{2}\alpha_{t-1}-\alpha_{t-2} \right)\left\|u_{t-1}-1 \otimes \bar{u}_{t-1}\right\|^{2}\right.\\
    &\left.+\alpha_{t-1}\left(1+\frac{1}{c_{3}}\right)\left[ 3 m(1-\eta)^{2} \sigma_{f}^{2}+3 m(1-\eta)^{2} C_{f}^{2}+3(1-\eta)^{2} mB^{2} \right]\right]
\end{align*}
Combining the above results, we have
\begin{align*}
    \mathbb{E}\left[ W_{t+1}-W_{t} \right]\leq &\mathbb{E}\left[ -\frac{\alpha_{t}}{2}\left\|\nabla l\left(\bar{x}_{t}\right)\right\|^{2}+\left[\frac{2 \alpha_{t}L_{f}^{2}}{m}-\frac{\beta_{t}L_{\mu_{g}}}{2} \right]\left\|y_{t}-y_{t}^{*}\right\|^{2}\right.\\
    &\left. + \left[ \frac{2\alpha_{t} L_{l}^{2}}{m}+\left( 1+c_{2} \right)\lambda^{2}-1 \right]\left\|x_{t}-1 \otimes \bar{x}_{t}\right\|^{2} \right.\\
    &\left. +\left[ \frac{4 L_{y}^{2} \alpha_{t}^{2}}{\beta_{t} L_{\mu_{g}}}+\left(1+\frac{1}{c_{2}}\right) \alpha_{t}^{2}+\left(1+c_{3}\right) \lambda^{2}\alpha_{t}-\alpha_{t-1} \right]\left\|u_{t}-1 \otimes \bar{u}_{t}\right\|^{2} \right.\\
    &\left. +\alpha_{t}\left[ 2B^{2}+5(1-\eta)^{2} m \sigma_{f}^{2}+3(1-\gamma)^{2} m \sigma_{g}^{2}+10\eta^{2}mB^{2} \right] \right.\\
    &\left. +\alpha_{t}\left(1+\frac{1}{c_{3}}\right)\left[3 m(1-\eta)^{2} \sigma_{f}^{2}+3 m(1-\eta)^{2} C_{f}^{2}+3(1-\eta)^{2} m B^{2}\right] \right]
\end{align*}
with the conditions as follows:
\begin{align*}
    &-\left(\frac{\alpha_{t}}{2}-\frac{L_{l} \alpha_{t}^{2}}{2}\right)+\frac{4 L_{y}^{2} \alpha_{t}^{2} m}{\beta_{t} L _{\mu_{g}}}+6 \gamma^{2} L_{g}^{2} \alpha_{t}^{3} m+5 \eta^{2} L_{f^{\prime}}^{2} \alpha_{t}^{3} m \leq 0 \\
    &12 \gamma^{2} L_{g_{y}}^{2} \beta_{t}^{2}\alpha_{t}-\frac{\beta_{t}}{\mu_{g}+L_{g}} \leq 0
\end{align*}
Therefore, the lemma is proved.
\end{proof}

\subsection{Proof of Theorem}

Telescoping the results in Step 6 from $0$ to $T-1$, we have 
\begin{equation*}
    \begin{aligned}
            \mathbb{E}\left[ W_{T}-W_{0} \right]\leq &\mathbb{E}\left[ -\sum_{t=0}^{T-1}\frac{\alpha_{t}}{2}\left\|\nabla l\left(\bar{x}_{t}\right)\right\|^{2}+\sum_{t=0}^{T-1}\alpha_{t}\left[ 5(1-\eta)^{2} m \sigma_{f}^{2}+3(1-\gamma)^{2} m \sigma_{g}^{2}+2B^{2}+10\eta^{2}mB^{2} \right] \right. \\
            &\left. +\sum_{t=0}^{T-1}\alpha_{t}\left( 1+\frac{1}{c_{3}} \right)\left[3 m(1-\eta)^{2} \sigma_{f}^{2}+3 m(1-\eta)^{2} C_{f}^{2}+3(1-\eta)^{2} m B^{2}\right] \right]
        \end{aligned}
\end{equation*}
with the conditions as follows:
\begin{equation*}
    \begin{aligned}
        &\frac{4 L_{y}^{2} \alpha_{t}^{2}}{\beta_{t} L_{\mu_{g}}}+\left(1+\frac{1}{c_{2}}\right) \alpha_{t}^{2}+\left(1+c_{3}\right) \lambda^{2}\alpha_{t}-\alpha_{t-1}\leq 0\\
        &\frac{2 \alpha_{t}L_{f}^{2}}{m}-\frac{\beta_{t}L_{\mu_{g}}}{2}\leq 0\\
        &\frac{2\alpha_{t} L_{l}^{2}}{m}+\left( 1+c_{2} \right)\lambda^{2}-1\leq 0
    \end{aligned}
\end{equation*}
Denote $C_{bias}=5(1-\eta)^{2} m \sigma_{f}^{2}+3(1-\gamma)^{2} m \sigma_{g}^{2}+\left( 1+\frac{1}{c_{3}} \right)\left[ 3(1-\eta)^{2} m \sigma_{f}^{2}+3(1-\eta)^{2} m C_{f}^{2} \right]$ and $C_{bias}^{'}=2+10\eta^{2}m+3\left( 1+\frac{1}{c_{3}} \right)\left( 1-\eta \right)^{2}m$. Dividing by $T$ on both sides, we get
\begin{align*}
    \frac{\mathbb{E}\left[ W_{T}-W_{0} \right]}{T}\leq &\mathbb{E}\left[ -\frac{1}{T}\sum_{t=0}^{T-1}\frac{\alpha_{t}}{2}\left\|\nabla l\left(\bar{x}_{t}\right)\right\|^{2}+\frac{1}{T}\sum_{t=0}^{T-1}\alpha_{t}C_{bias}+\frac{1}{T}\sum_{t=0}^{T-1}\alpha_{t}C_{bias}^{'}B^{2} \right]
\end{align*}

Since $\alpha_{t}:=\left( \omega+t \right)^{-1/3}$, we have $\alpha_{T}\le \alpha_{t},\;\forall t\in \left\{ 0,\ldots,T-1  \right\}$. Multiplying by $2/\alpha_{T}$ and rearranging the terms, we have
\begin{equation*}
    \begin{aligned}
        \mathbb{E}\left[ \frac{1}{T} \sum_{t=0}^{T-1}\|\nabla l(\bar{x}_{t})\|^{2} \right] \leq & \mathbb{E}\left[ \frac{2\left(W_{0}-l^{*}\right)}{\alpha_{T} T} +\frac{2}{\alpha_{T} T} \sum_{t=0}^{T-1} \alpha_{t}C_{bias}+\frac{2}{\alpha_{T} T} \sum_{t=0}^{T-1} \alpha_{t}C_{bias}^{'}B^{2} \right]
    \end{aligned}
\end{equation*}
With the definition of $\alpha_{t}$ and choose $\omega$ satisfies $\sum_{t=0}^{T-1}\alpha_{t}\le \log\left( T+1 \right)$. With the definition of the potential function $W_{t}$, we have 
\begin{align*}
    \mathbb{E}\left[ W_{0} \right]&=\mathbb{E}\left[ l\left(\bar{x}_{0}\right)+\left\|y_{0}-y_{0}^{*}\right\|^{2}+\alpha_{-1}\left\|e_{0}^{f}\right\|^{2}+\alpha_{-1}\left\|e_{t}^{g}\right\|^{2}+\left\|x_{0}-1 \otimes \bar{x}_{0}\right\|^{2}+\alpha_{0-1}\left\|u_{0}-1 \otimes \bar{u}_{0}\right\|^{2} \right]\\
    &\le \mathbb{E}\left[ l\left(\bar{x}_{0}\right)+\left\|y_{0}-y_{0}^{*}\right\|^{2}+\left\|x_{0}-1 \otimes \bar{x}_{0}\right\|^{2}+\alpha_{-1}\left\|u_{0}-1 \otimes \bar{u}_{0}\right\|^{2}+\alpha_{-1}\sigma_{f}^{2}+\alpha_{-1}\sigma_{g}^{2} \right]
\end{align*}
Denote $\mathfrak{B}_{t}=l\left(\bar{x}_{t}\right)+\left\|y_{t}-y_{t}^{*}\right\|^{2}+\left\|x_{t}-1 \otimes \bar{x}_{t}\right\|^{2}+\alpha_{t-1}\left\|u_{t}-1 \otimes \bar{u}_{t}\right\|^{2}$. Use the fact that $B=1/T$ when choose $K=\left( \mu_{g}/L_{g} \right)\log\left( C_{g_{xy}}C_{f_{y}}T/\mu_{g} \right)$. Then, we have the following convergence results:
\begin{equation*}
    \begin{aligned}
        \frac{1}{T}\sum_{t=0}^{T-1}\mathbb{E}\left[ \left\| \nabla l\left( \bar{x}_{t} \right) \right\| ^{2}\right]&\le \frac{2}{\alpha_{T}T}\mathbb{E}\left[ \mathfrak{B}_{0}-l^{*} \right]+\frac{2}{\alpha_{T}T}\left(\alpha_{-1}\sigma_{f}^{2}+\alpha_{-1}\sigma_{g}^{2} \right)\\
        &+\frac{2\log\left( T+1 \right)}{\alpha_{T}T}C_{bias}+\frac{2\log\left( T+1 \right)}{\alpha_{T}T^{3}}C_{bias}^{'}
    \end{aligned} 
\end{equation*}
Hence, the theorem is proved.
